# Supplementary material for: Single-atom dopants in plasmonic nanocatalysts
Source: arXiv:2301.08217 ancillary file (2023-01-19)
Supplement: Supplementary file 1 [file Supplementary_Information.pdf]

Supplementary Information

# Single-atom dopants in plasmonic nanocatalysts

Daniel Sorvisto, Patrick Rinke, and Tuomas P. Rossi

*Department of Applied Physics, Aalto University, Espoo, Finland*

## Contents

**Supplementary Figures** **2**

S1. Effect of the pulse direction . . . 2
S2. Change in photoabsorption spectrum due to the dopant atom . . . 2
S3. Change in density of states due to the dopant atom . . . 3
S4. Change in hot-carrier distribution due to the dopant atom . . . 3
S5. Hot-carrier generation in 201-atom particles with facet dopant atom . . . 4

## Supplementary Figures

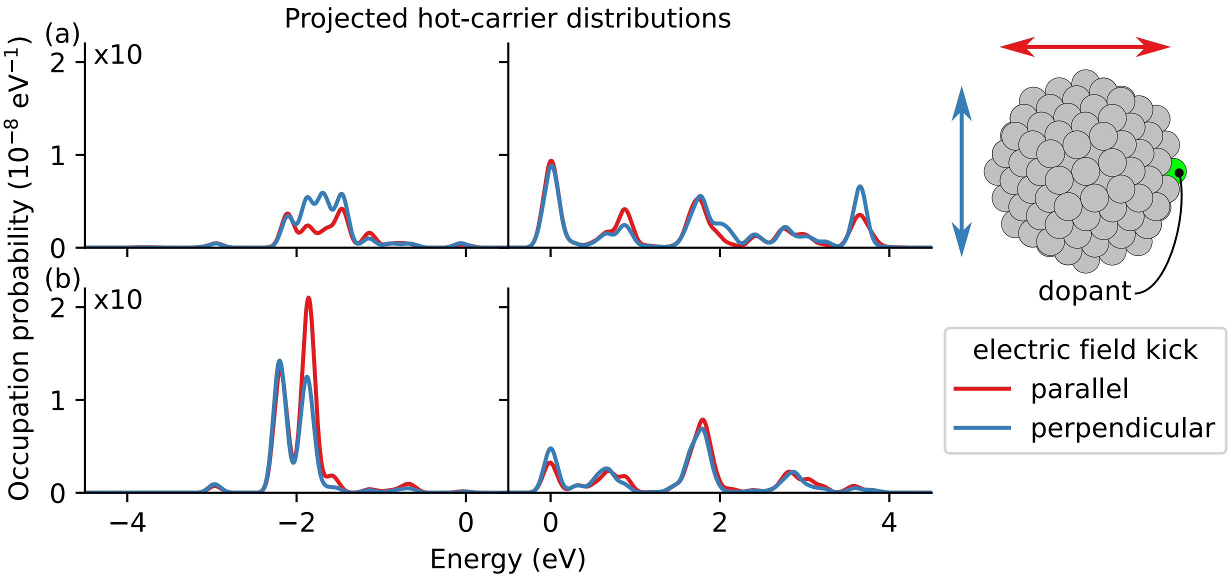


**Supplementary Figure S1: Effect of the pulse direction.** Hot-carrier distributions projected to the dopant atom in (a) $Ag_{201}$/Pt(corner) and (b) $Ag_{201}$/Pt(facet) for the pulse electric field aligned parallel or perpendicular to the axis that connects the center of the particle with the dopant atom. The orientation of the particle with respect to the electric field perturbation affects the quantitative results, but the order of magnitude and the qualitative results appear to be unaffected.

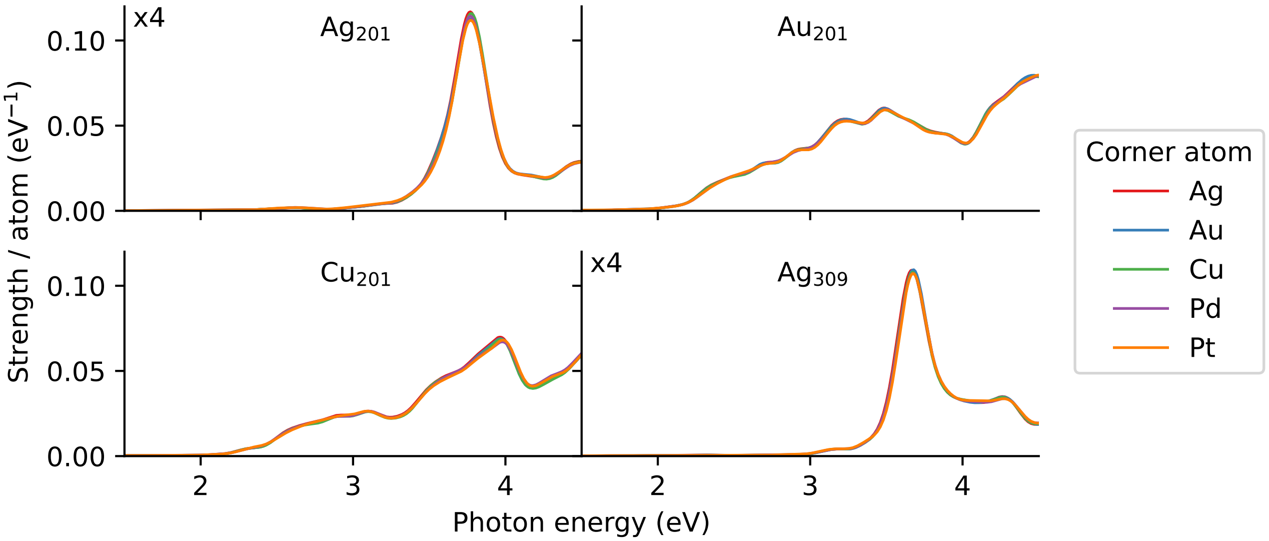


**Supplementary Figure S2: Change in photoabsorption spectrum due to the dopant atom.** Photoabsorption spectra of $Ag_{201}$, $Au_{201}$, $Cu_{201}$, and $Ag_{309}$ nanoparticles with the corner atom replaced with Ag, Au, Cu, Pd, or Pt. Note that the y-axis limits have an indicated multiplier.

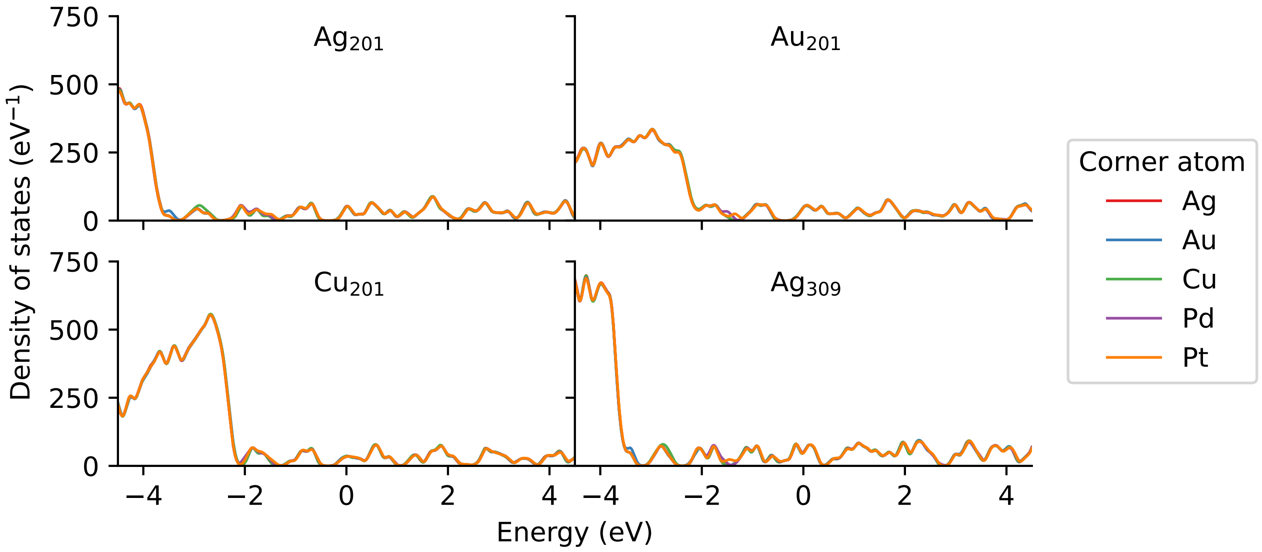


**Supplementary Figure S3: Change in density of states due to the dopant atom.** Density of states of $Ag_{201}$, $Au_{201}$, $Cu_{201}$, and $Ag_{309}$ nanoparticles with the corner atom replaced with Ag, Au, Cu, Pd, or Pt.

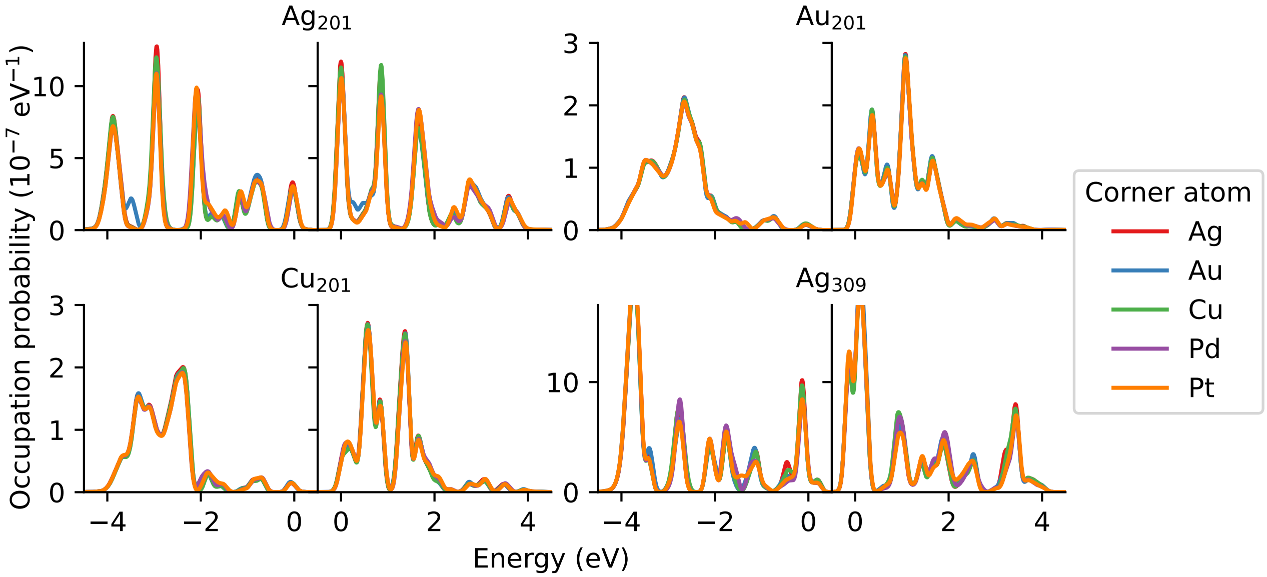


**Supplementary Figure S4: Change in hot-carrier distribution due to the dopant atom.** Hot-carrier distributions of $Ag_{201}$, $Au_{201}$, $Cu_{201}$, and $Ag_{309}$ nanoparticles with the corner atom replaced with Ag, Au, Cu, Pd, or Pt.

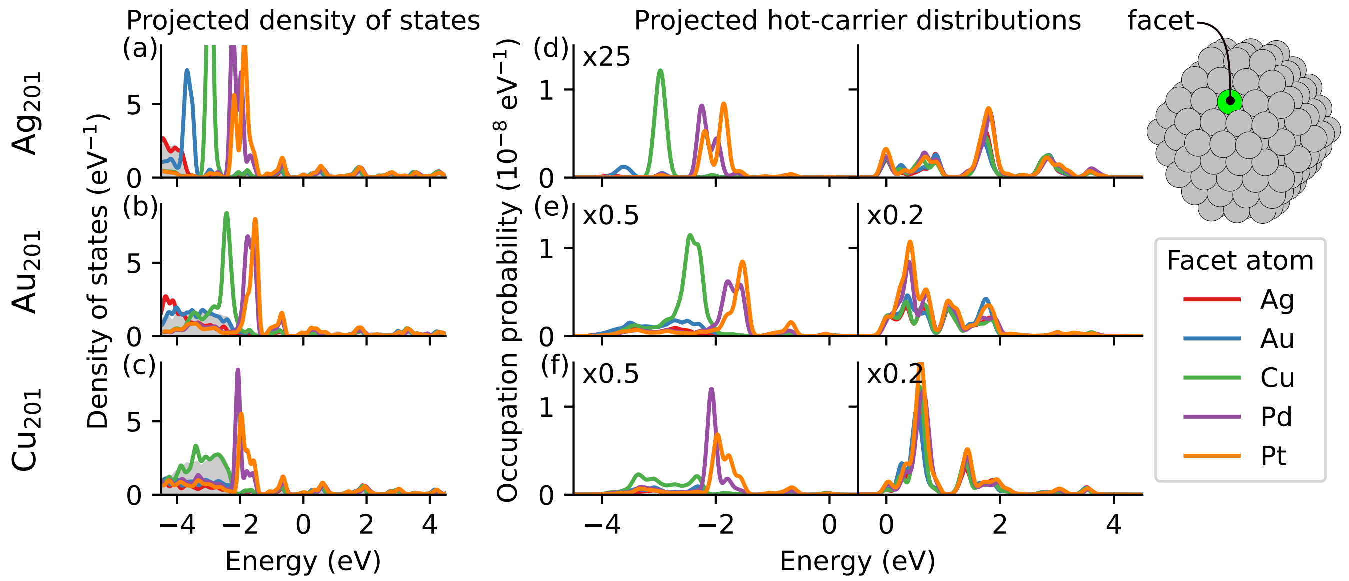


**Supplementary Figure S5: Hot-carrier generation in 201-atom particles with facet dopant atom.** (a-c) Density of states and (d-f) hot-carrier distributions projected to the facet atom in $Ag_{201}$, $Au_{201}$, and $Cu_{201}$ nanoparticles with the same facet atom replaced with Ag, Au, Cu, Pd, or Pt. The figure is analogous to Fig. 2 in the main paper.
